# Supplementary material for: Learning Graph Search Heuristics
Source: arXiv:2212.03978 source file (2023-01-11)
Supplement: Supplementary file 1 [file appendix.tex]

\documentclass{article}
\usepackage{log_2022}   % for anonymous submission
% \usepackage{log_2022}         % for camera-ready version
% \usepackage[preprint]{log_2022}
%                               % for preprint version
% \usepackage[eatrack]{log_2022}
%                               % for accepted extended abstracts

\usepackage{booktabs}           % professional-quality tables
\usepackage{multirow}           % tabular cells spanning multiple rows
\usepackage{multicol}
\usepackage{amsfonts}           % blackboard math symbols
\usepackage{graphicx}           % figures
\usepackage{duckuments}         % sample images
\usepackage{array}
\usepackage{lipsum}
\usepackage{subcaption}
\usepackage{wrapfig}

\usepackage[utf8]{inputenc} % allow utf-8 input
\usepackage[T1]{fontenc}    % use 8-bit T1 fonts
\usepackage{url}            % simple URL typesetting
\usepackage{nicefrac}       % compact symbols for 1/2, etc.
\usepackage{microtype}      % microtypography

% If you want to use natbib:
\usepackage[numbers,compress,sort]{natbib}
%                               % for numerical citations
% \usepackage[sort,round]{natbib}
%                               % for textual citations

% If you want to use bibLaTeX:
% \usepackage[
%      backend=biber,
%      style=numeric-comp,
%      backref=true,
%      natbib=true]{biblatex}
% \addbibresource{reference.bib}

\usepackage[mathscr]{euscript}
\usepackage[export]{adjustbox}

\usepackage{enumitem}

\usepackage[ruled,vlined]{algorithm2e}  %updated version of algorithm2e.sty is in ./ folder.
\SetKwComment{Comment}{$\triangleright$\ }{}

\usepackage{amsmath,amssymb}

 % expected value

\title[Submission Guidelines and Formatting Instructions for LoG Conference 2022]{Learning Graph Search Heuristics}

\begin{document}

\appendix
\input{006appendix}

\end{document}
